# Supplementary material for: Explainable fMRI-based Brain Decoding via Spatial Temporal-pyramid Graph Convolutional Network
Source: arXiv:2210.05713 source file (2022-10-08)

# Emotion processing

L

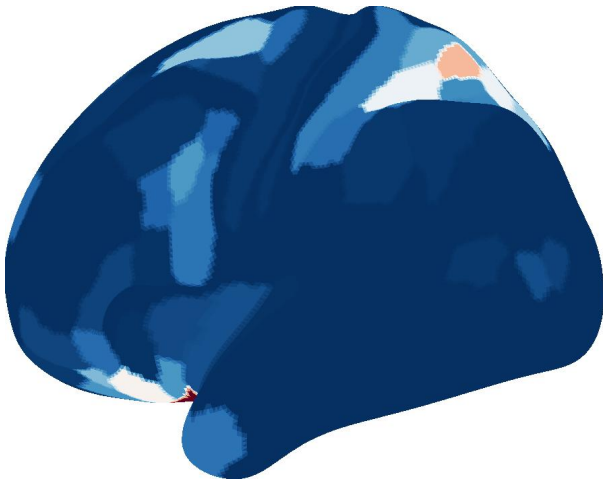

R

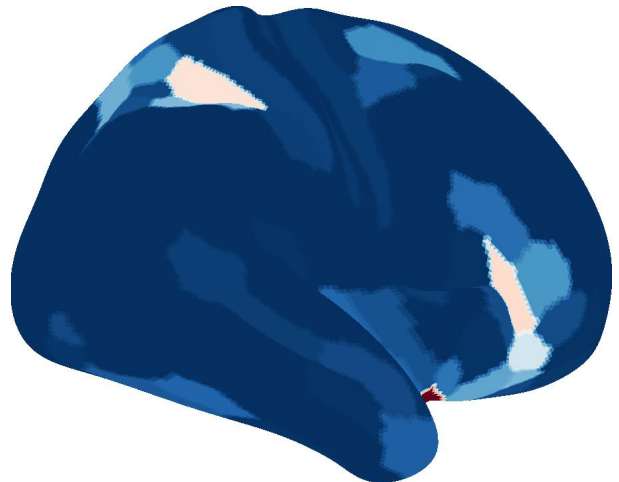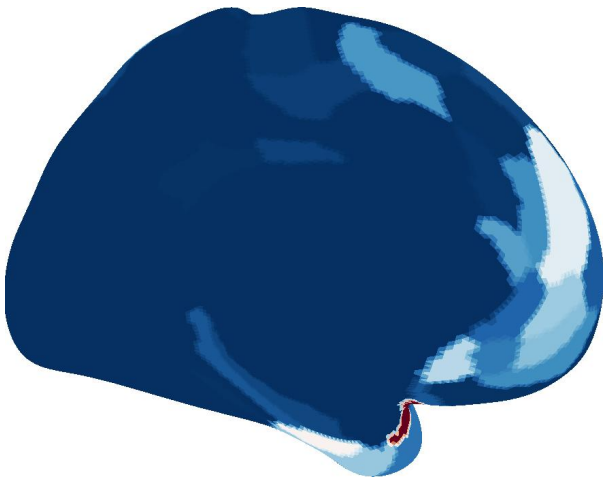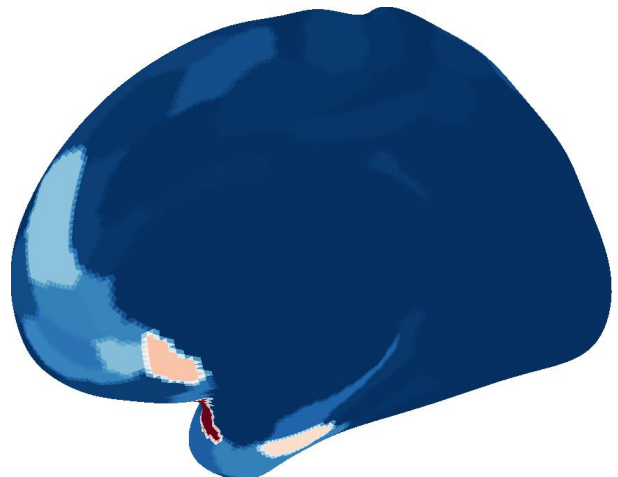

# Gambling

L

R

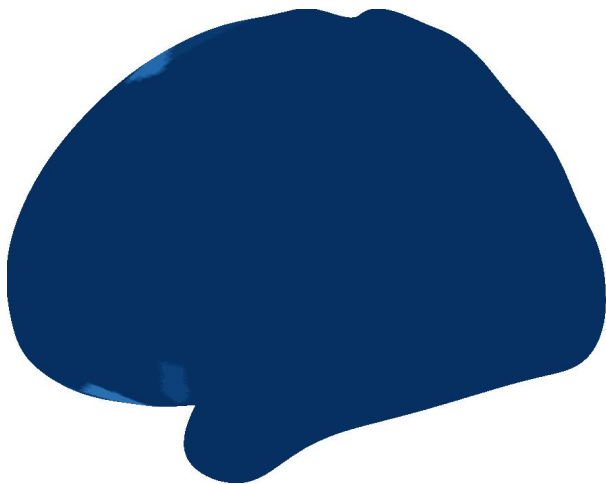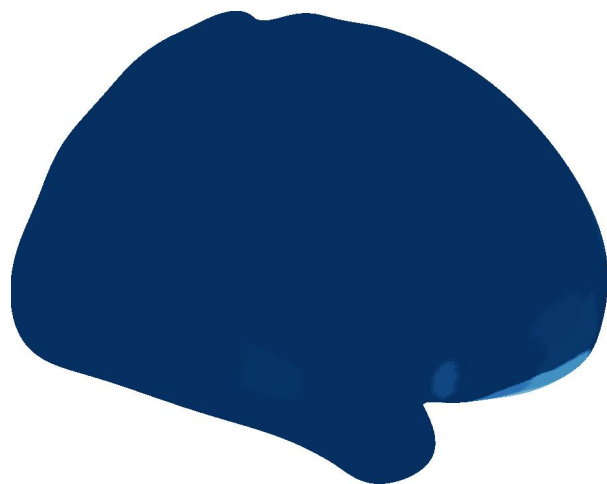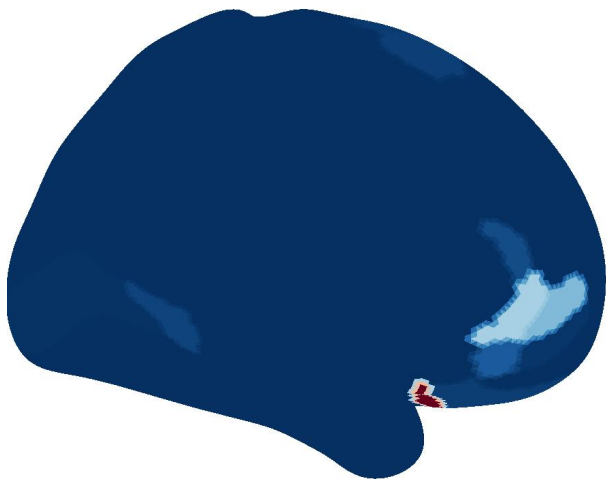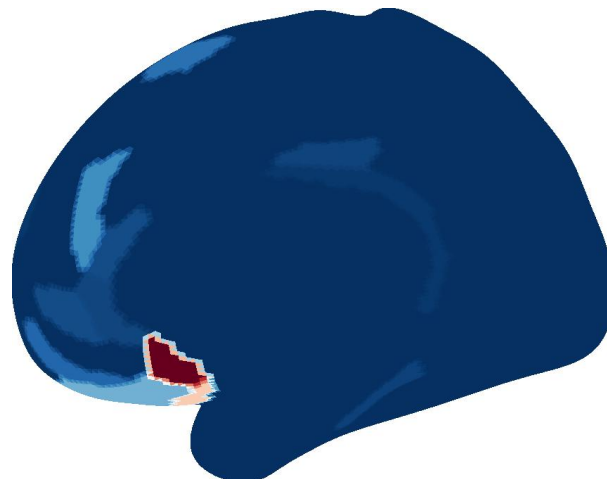

# Language

L

R

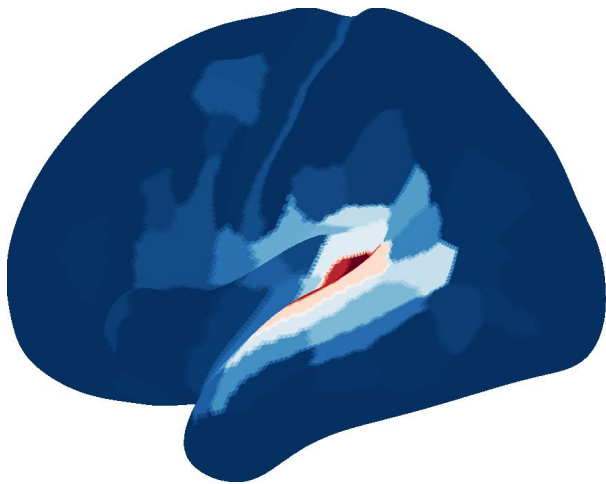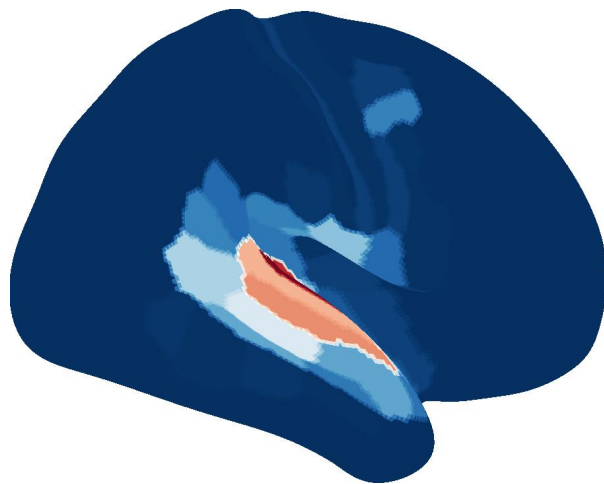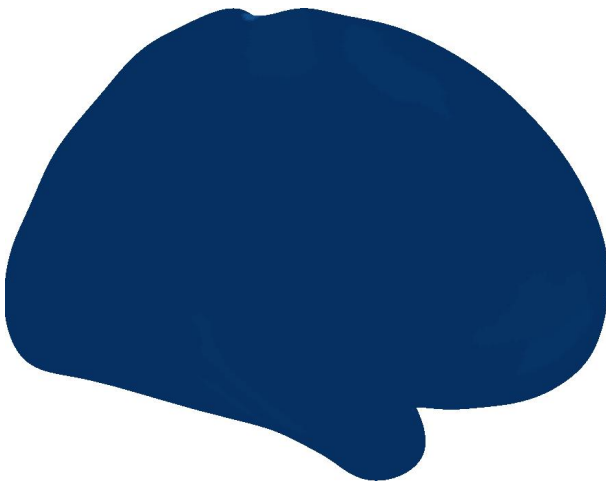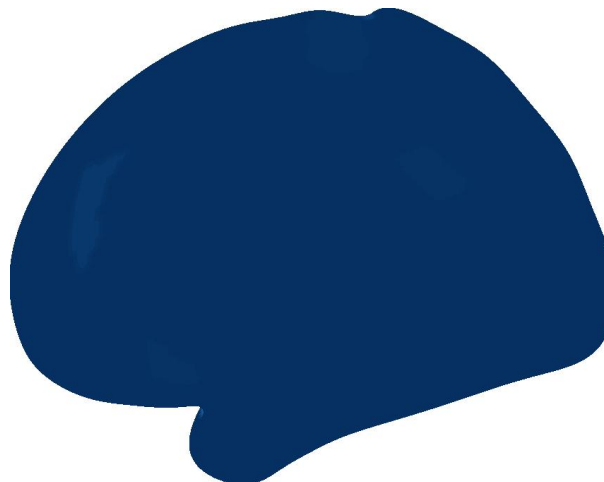

# Motor

L

R

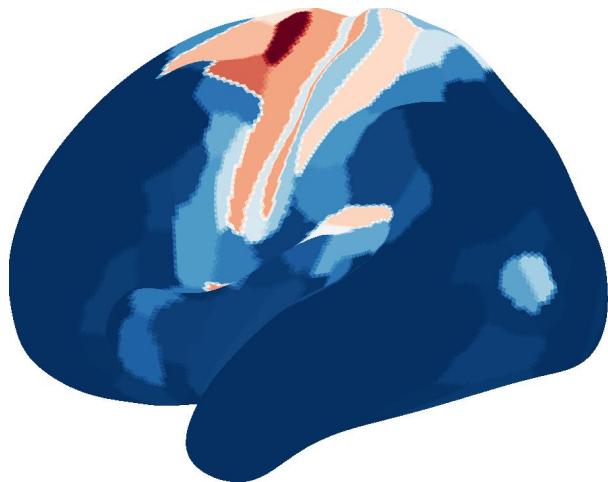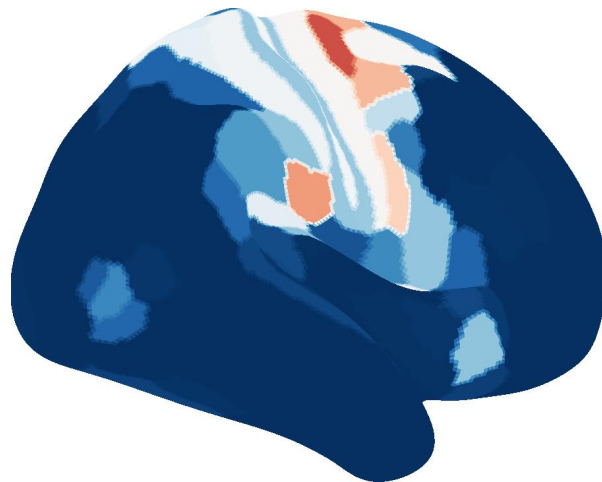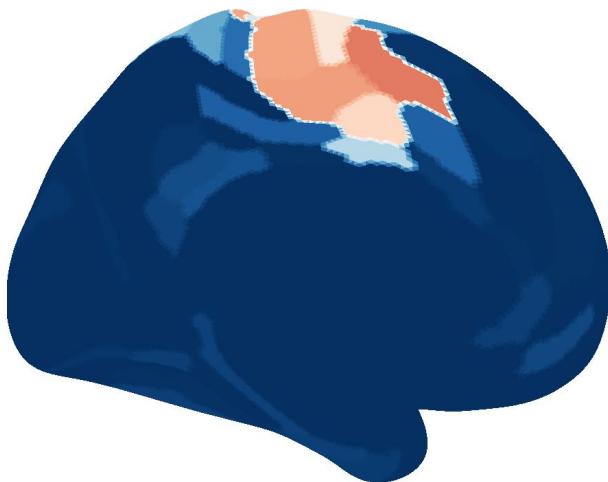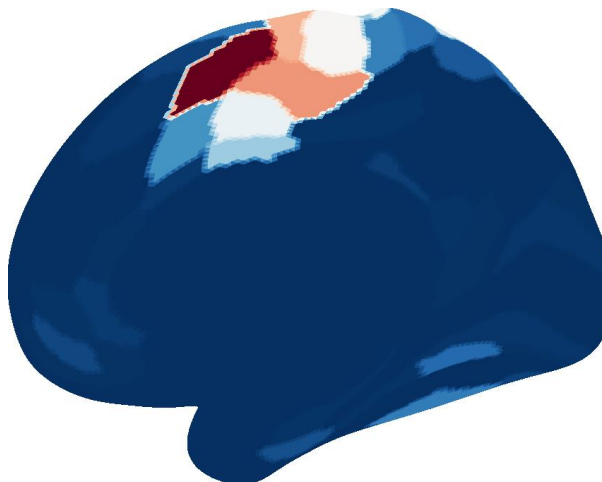

# Social cognition

L

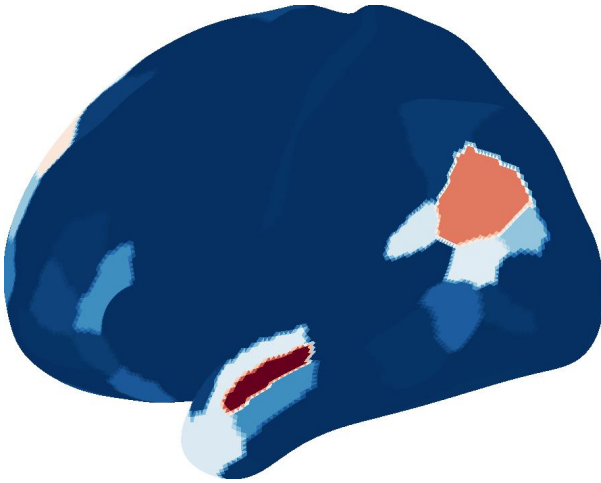

R

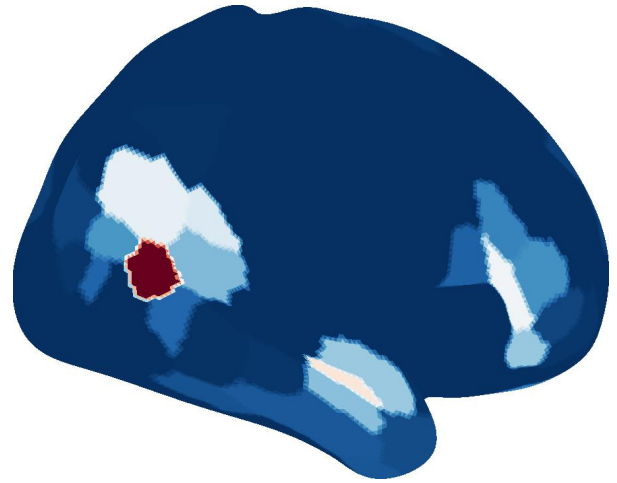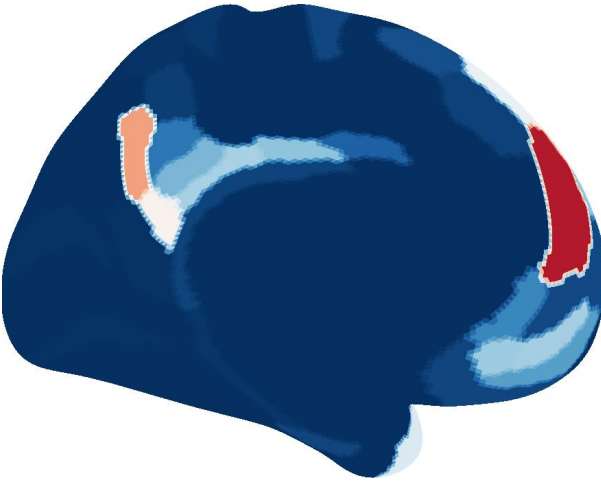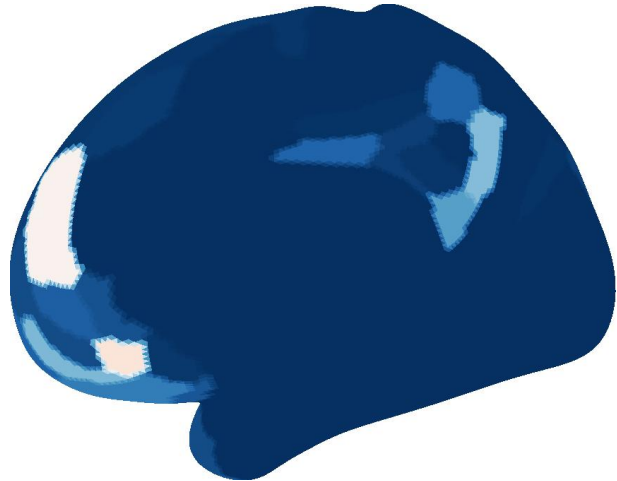

# Relational processing

L

R

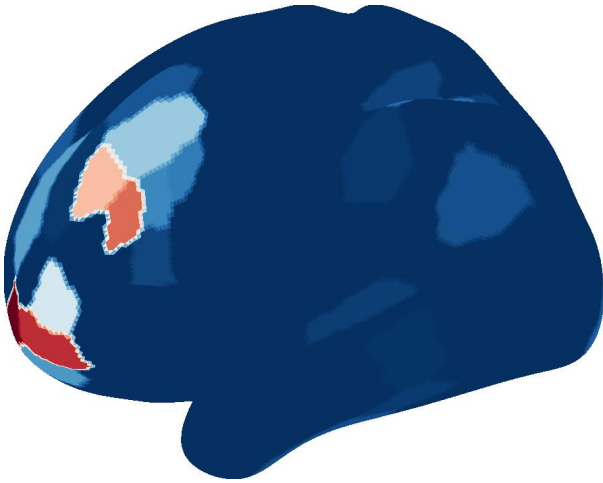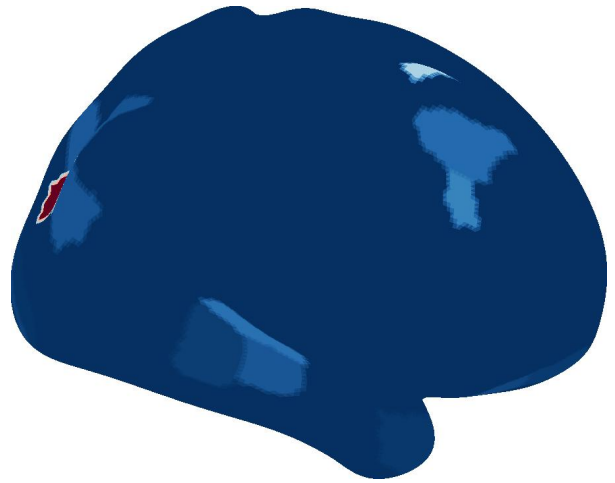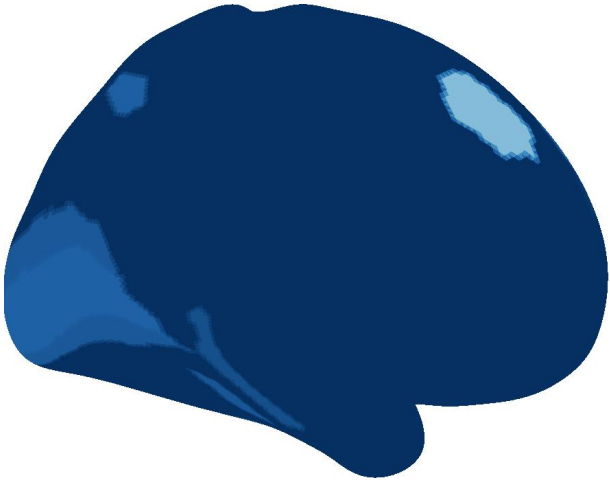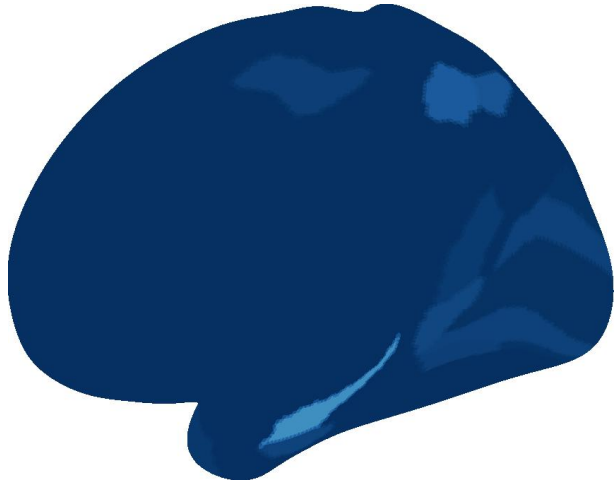

# Working memory

L

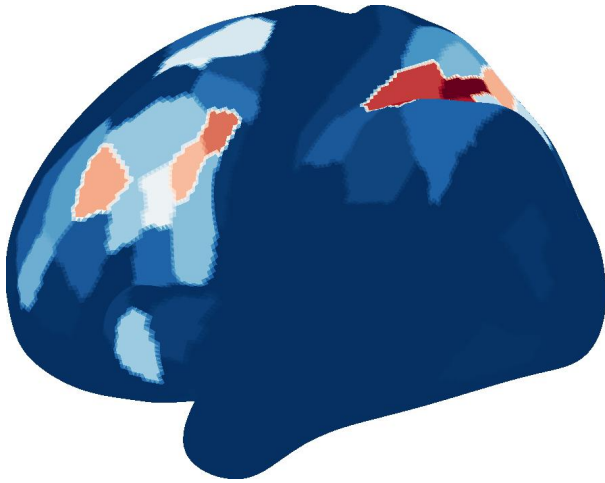

R

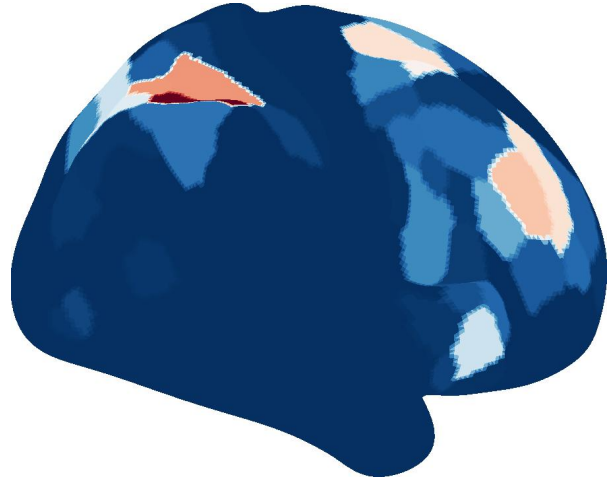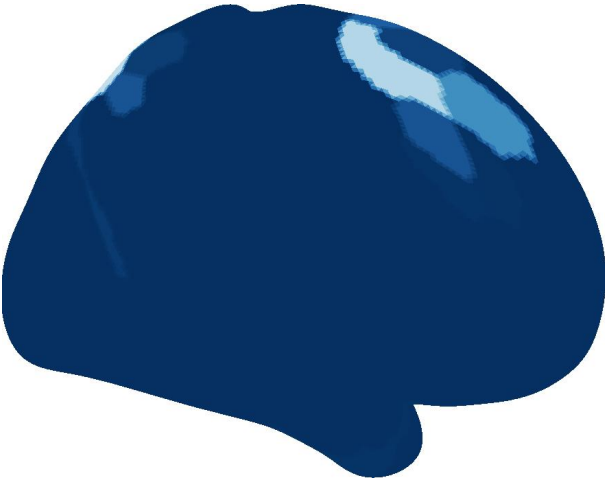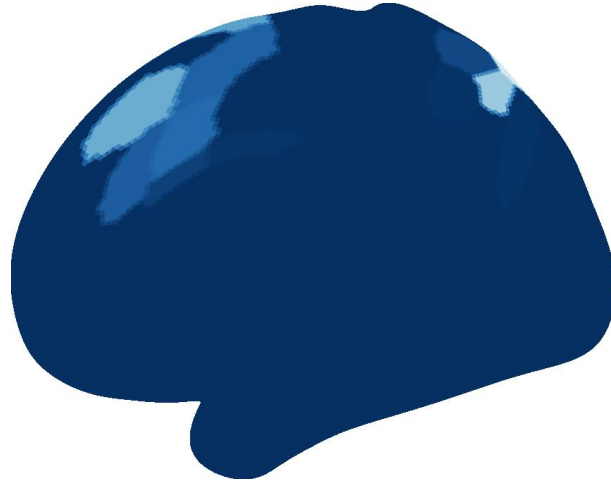

Supplement: Supplementary file 1 [file groundtruth.pdf]
